# Supplementary material for: Cognitive Ability and Tournament Entry: Evidence from Three Korean Populations
Source: arXiv:2108.08097 source file (2026-08-14)
Supplement: Supplementary file 1 [file Online_Appendix.pdf]

For Online Publication

Online Appendices

# Why North Korean Refugees are Reluctant to Compete: The Roles of Cognitive Ability

## Experimental Instructions in Korean and English

주관기관  
서울대학교

조사기관  
nielsen

의사결정에 관한 경제학 실험 및 설문조사

연구목적 및 내용

본 연구는 경제 의사결정 과정에 대해 알아보고자 하는 목적으로 서울대학교가 한국연구재단의 지원을 받아 실시하는 경제학 실험 연구입니다. 대한민국에 거주하는 다양한 성인 그룹을 대상으로 경제 의사결정 과정에 대해 실험과 설문조사를 통해 알아보고, 관련 연구의 기초자료로 활용하고자 합니다.

연구절차 및 방법

본 연구는 다음 2개의 파트로 구성되어 있으며, 약 2시간 30분 가량 소요될 예정입니다.  
실험 단계에 따라 컴퓨터와 종이 조사표를 번갈아 가며 진행하오니, 진행자의 설명에 따라 주시기 바랍니다.

1) 실험파트 : 총 4단계의 실험이 진행되며, 앞 3단계별 선생님의 성과와 선택 등에 따라 선생님이 오늘 받으실 답례금이 책정됩니다. 마지막 4단계 실험은 답례금 결정에 영향을 주지 않습니다.

2) 설문파트 : 선생님의 경제활동과 인식 등을 묻으며, 약 40~50분 정도 소요가 예상됩니다.

귀하께서 설문조사까지 마치면, 기본 답례금에 실험을 통해 확보하신 금액을 덧붙여 나가실 때 지급해 드립니다.  
구체적인 실험 내용과 방법은 각 단계별로 설명을 드리도록 하겠습니다.

개인정보보호

실험 참석 확인을 위해 보유한 선생님의 정보(이름, 전화번호, 성, 연령 등)와 이 자리에서 응답하신 선생님의 모든 정보는 실험 종료와 동시에 모두 폐기되며, 통계법 제33~34조에 의해 통계적 목적으로만 사용되고, 비밀은 엄격히 보호됩니다.

본 연구는 서울대학교 생명윤리심의위원회의 승인을 받았습니다. (IRB No. 1506/002-001, 승인날짜 2015.6.3)

### Purpose of study

This study is conducted by a research team at Seoul National University with the support of the National Science Foundation of Korea to understand economic decision making. We recruit a variety of South Korean residents to take part in economics experiments about decision making and survey. The collected data will be served as basic materials for academic research.

### Procedure and method

This study consists of the following two parts and will take approximately 2.5 hours to complete. The experiments and survey will be computer-based and paper-based. Please follow instructions given by the experimenter.

1) Experiment part: It consists of four stages. Your earnings in this study will depend on your performance and choices in the first three stages. The last stage will not affect your earnings.

2) Survey part: You will answer survey questions of economic activities and attitudes, it will take about 40~50 minutes to complete.

If you have completed the study, you will receive your earnings and a show-up fee before you leave. We will give you specific instructions about each stage of the study when it starts.

### Privacy

All the personal information, including name, phone number, gender, age, etc., and the responses you give in this study will be discarded when this research is completed. In accordance with the Article 33-34 of the Statistics Act, all confidential information is strictly protected and used only for the purpose of statistics.

This research has been approved by the Institutional Review Board at Seoul National University (IRB No. 1506/002-001, Approval date: June 3, 2015).

## PART A

# 보수책정 1단계

- ❖ 개인 실험은 총 3개의 실험으로 이루어집니다.
- ❖ 각 단계별로 문제를 풀어 맞춘 개수와 각 단계별 차별적인 보수선택 방식에 따라 단계별 선생님의 보수가 결정되며, 3개 실험으로 결정된 보수 중 무작위로 한 개를 선택해 선생님의 최종 보수가 결정됩니다.

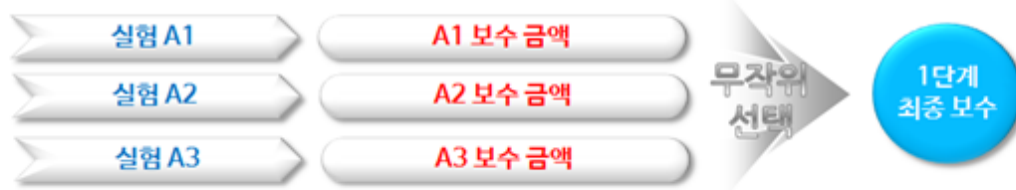

- ❖ 최종 보수가 결정되면 그 금액에 기본 참가비(5만원)를 덧붙여 모든 설문이 끝나고 나가실 때 지급됩니다.
- ❖ 각 단계별 실험과 보수 결정 방식은 순서대로 단계 시작 전에 설명 드리겠습니다.

### Part A: Earnings

The experiment will consist of 3 stages. Your earnings in each stage will depend on the number of correct answers in problem solving and an incentive scheme. Your final earnings will be determined by a random selection of your earnings in the three stages. You will receive this randomly selected final earnings together with a participation fee (50,000 KRW) when you leave after completing the study.

We will give you an information of the detail of each stage experiment and an incentive scheme when it starts.

## 실험 A1 성과제

- ❖ 보수책정 1단계 모든 실험은 선생님이 맞추신 퀴즈의 정답 수에 따라 보수액이 결정됩니다.
- ❖ 다만 보수책정 방식에 있어 차이가 있으며 첫번째는 맞추신 수 그대로 보수가 결정되는 **성과제**입니다.
- ❖ 선생님께서 앞으로 받으실 봉투 안에는 **총 20개의 숫자표**가 들어 있습니다.
- ❖ **총 5분** 동안 각 숫자표에 있는 “0”의 개수를 맞추는 것이 문제이며, 맞추신 개수에 따라 **보수액이 결정**됩니다.

### Experiment A1: Piece rate scheme

In all stages of the experiment, your earnings will depend on the number of your correct answers in a task. In the first stage, your earnings will depend solely on the number of your correct answers.

You will receive an envelope containing 20 tables and will be asked to answer the number of “0” in each table.

- ❖ 아래 숫자 표에서 0의 개수를 맞춰주세요.
- ❖ 총 20개의 숫자 표가 있습니다.

[숫자 표 A1-1]

|   |   |   |   |   |   |   |
|---|---|---|---|---|---|---|
| 0 | 1 | 0 | 1 | 0 | 0 | 0 |
| 1 | 1 | 1 | 0 | 0 | 1 | 0 |
| 0 | 1 | 0 | 1 | 1 | 0 | 0 |
| 1 | 0 | 1 | 0 | 1 | 0 | 1 |
| 0 | 0 | 1 | 1 | 1 | 0 | 0 |
| 0 | 1 | 0 | 0 | 0 | 1 | 0 |
| 1 | 1 | 0 | 1 | 1 | 0 | 0 |

- ❖ 답을 컴퓨터의 화면 응답란에 입력해주세요.
- ❖ 숫자표 순서가 틀리지 않도록 주의해주세요.  
순서가 틀리면 오답이 됩니다.
- ❖ 옆의 숫자표의 0의 개수는 27개입니다.

27

Q8. '숫자표 [A1-1]'에서 숫자 '0'의 개수를 맞춰주세요.

선생님의 응답  개

As an example, please count the number of zeros in the table below [Number Table A1-1]. You will then be asked to submit your answer. Please bear in mind the order of Number Table. The answer in this example is 27.

You will face such 20 tables.

### 실험 A1의 보수 결정

- ❖ 첫 번째 단계의 보수는 선생님께서 맞추신 정답 \* 1천원을 받게 됩니다.
- ❖ 3개를 맞추면 3천원, 12개를 맞추면 1만 2천원 등이며, 다 맞추면 2만원, 하나도 맞추지 못하면 0원입니다.

정답의 개수 \* 1천원

3개 맞추 경우 3,000원

12개 맞추 경우 12,000원

- ❖ 문제를 한 개씩 푸실 때마다 문제의 정답이 공개되며,  
모든 문제를 다 풀고 나면 선생님께서 맞추신 정답 개수와 첫 번째 보수 금액을 확인할 수 있습니다.

#### Earnings in Experiment A1

You will receive 1,000 KRW for each correct answer. For instance, if you solved 3 tables correctly, you will receive 3,000 KRW. If you solved 12 tables correctly, you will receive 12,000 KRW. If you did not solve any table correctly, you will earn nothing.

Once you submit your answer in each table, you will be informed of a correct answer. After you solved all the tables, you will be informed of the number of your correct answers and your earnings in this stage.

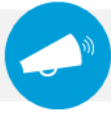

진행요원들은 연습 숫자표를 수거해 주세요.

(반납이 끝나면)

- ❖ 잠시 후 숫자표 20개가 들어 있는 문제 봉투를 나누어 드리겠습니다.
- ❖ 진행자가 '시작'을 외치면 총 5분 동안 문제를 푸시고 정답을 입력해주세요.  
시작을 외치기 전 봉투를 미리 개봉하면 실격 처리 됩니다.
- ❖ 숫자표에 정답을 적어 두셨다가 컴퓨터에 입력하셔도 관계 없으며,  
다만 시간 안에, 반드시 정답을 컴퓨터에 입력해야 점수가 계산됩니다.
- ❖ 진행자 화면에 시간이 보일 예정이며, 1분이 남으면 알려드릴 예정이니 입력을 반드시 완료해주세요.
- ❖ 5분이 모두 지나면 봉투는 한꺼번에 모두 회수하겠습니다.

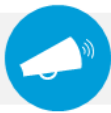

진행요원들은 숫자표 봉투 A1을 나눠주세요.

- ❖ 먼저, 봉투에 본인 이름과 ID를 정확히 적어주세요.
- ❖ 그럼, 이제 시작을 외치면 '다음'을 누르시고 봉투를 개봉해 5분간 문제풀이를 시작하게 됩니다.

“시작”

You will soon be given an envelope containing 20 tables. If the experimenter announces “Start”, you can start counting zeros and submitting your answers in 5 minutes.

You will be disqualified if you open your envelope before the experimenter announces “Start.” Answers you submit within 5 minutes in the computer will be only counted.

The experimenter will show you a timer through a beam projector and will announce “one minute remaining” when 4 minutes pass.

[The experimental assistants distribute envelopes to subjects]

Please write down your name and ID on the envelope. The experimenter is about to announce “Start.”

실험A1을 종료합니다.

진행자에게 문제지와 봉투를 제출해주세요.

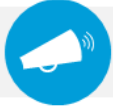

진행요원들은 담당구역의 봉투를 신속하게 걷어주세요.  
앞에 비치된 A1 수거 상자에 모아주세요.

아래 “다음” 버튼을 누르시면 **정답의 총 개수**와

선생님의 개인실험 1단계 **보수 금액이 공개** 됩니다.

Experiment A1 has just ended. Please submit your envelope and tables to the experimenter.

If you press “Next” button in your computer, you will be informed of the number of correct answers and your earnings in this stage.

## 실험 A2 경쟁제

- ❖ 두 번째 단계인 경쟁제도 첫 단계와 동일하게 5분 안에 20개의 문제를 풀게 됩니다.
- ❖ 그러나 보수는 첫 단계처럼 선생님이 맞추신 금액에 따라 결정되지 않습니다.
- ❖ 선생님과 실험에 참여하고 있는 다른 사람과 무작위로 짝을 지어 드리며,  
선생님과 짝은 동일한 문제를 풀게 됩니다.
- ❖ 그 중 더 많이 맞춘 이긴 사람에게만 보수를 지급하며, 진 사람은 아무런 보수가 책정되지 않습니다.

### Experiment A2: Tournament scheme

In the second stage you will be again asked to solve 20 tables within 5 minutes. You will be randomly paired with another subject in the experiment. Each of you and your partner will receive an envelope containing the same set of 20 tables. One who solves a higher number of correct answers will become a winner and receive earnings. The other who loses (that is, solves a lower number of correct answers) will receive nothing.

- ❖ 아래 숫자 표에서 0의 개수를 맞춰주세요.
- ❖ 총 20개의 숫자 표가 있습니다.

[숫자 표 A1-1]

|   |   |   |   |   |   |   |
|---|---|---|---|---|---|---|
| 0 | 1 | 0 | 1 | 0 | 0 | 0 |
| 1 | 1 | 1 | 0 | 0 | 1 | 0 |
| 0 | 1 | 0 | 1 | 1 | 0 | 0 |
| 1 | 0 | 1 | 0 | 1 | 0 | 1 |
| 0 | 0 | 1 | 1 | 1 | 0 | 0 |
| 0 | 1 | 0 | 0 | 0 | 1 | 0 |
| 1 | 1 | 0 | 1 | 1 | 0 | 0 |

- ❖ 답을 컴퓨터의 화면 응답란에 입력해주세요.
- ❖ 숫자표 순서가 틀리지 않도록 주의해주세요.  
순서가 틀리면 오답이 됩니다.
- ❖ 옆의 숫자표의 0의 개수는 27개입니다.

27

Q8. '숫자표 [A1-1]'에서 숫자 '0'의 개수를 맞춰주세요.

선생님의 응답  개

As an example, please count the number of zeros in the table below [Number Table A1-1]. You will then be asked to submit your answer. Please bear in mind the order of Number Table. The answer in this example is 27.

You will face such 20 tables.

### 실험 A2 보수 결정

- ❖ 두 번째 단계의 보수는 선생님께서 다른 누군가와 경쟁을 해 이길 경우만 받을 수 있습니다.
- ❖ 맞춘 개수가 적어 경쟁에서 진 경우는 아무런 보수도 책정되지 않습니다(0원).
- ❖ 단, 이긴 사람은 맞춘 정답 \* 2천원으로 첫 단계의 두 배를 받게 됩니다.
- ❖ 단, 정답의 개수가 같으면 이긴 사람과 진 사람은 무작위로 결정됩니다.

| 내가 이길 경우                                |   | 내가 질 경우                                 |         |   |           |
|-----------------------------------------|---|-----------------------------------------|---------|---|-----------|
| 내 정답 12개                                | ➡ | 상대 정답 9개                                | 내 정답 7개 | ⬅ | 상대 정답 10개 |
| 내 보수 12개 * 2,000원 ➡ 24,000원<br>상대 보수 0원 |   | 내 보수 0원<br>상대 보수 10개 * 2,000원 ➡ 20,000원 |         |   |           |

- ❖ 다만, 이기고 지고는 모든 실험이 끝나고 프로그램을 통해 짝짓기가 이루어져 결정되며,  
모든 설문이 끝나고 밖으로 나가서 답례금을 받으실 때 상황판에서 확인하실 수 있습니다.

#### Experiment A2: Earnings

In this stage, you will receive earnings only if you win the competition against another subject. If you solve less tables correctly, you will receive nothing. If you win, you will receive 2,000 KRW for each correct answer, which is twice compared to 1,000 KRW earning in the first stage. When the number of correct answers is equal between you and your partner, a winner will be randomly selected.

You will be informed of whether you are a winner in this stage when you complete the study.

- ❖ 잠시 후 문제 봉투를 나누어 드리겠습니다.
- ❖ 진행자가 '시작'을 외치면 총 5분 동안 문제를 푸시고 정답을 입력해주세요.  
시작을 외치기 전 봉투를 미리 개봉하면 실격 처리 됩니다.
- ❖ 5분이 모두 지나면 봉투는 한꺼번에 모두 회수하겠습니다.

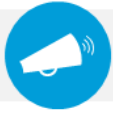

진행요원들은 숫자표 봉투 A1-2를 나눠주세요.

- ❖ 먼저, 봉투에 본인 이름과 ID를 정확히 적어주세요.
- ❖ 그럼, 이제 시작을 외치면 '다음'을 누르시고 봉투를 개봉해 5분간 문제풀이를 시작하게 됩니다.

## “시작”

You will soon be given an envelope containing 20 tables for this stage. If the experimenter announces “Start”, you can start counting zeros and submitting your answers in 5 minutes.

You will be disqualified if you open your envelope before the experimenter announces “Start.” Answers you submit within 5 minutes in the computer will be only counted.

The experimenter will show you a timer through a beam projector and will announce “one minute remaining” when 4 minutes pass.

[The experimental assistants distribute envelopes to subjects]

Please write down your name and ID on the envelope. The experimenter is about to announce “Start.”

실험A2를 종료합니다.

진행자에게 문제지와 봉투를 제출해주세요.

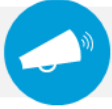

진행요원들은 담당구역의 봉투를 신속하게 걷어주세요.  
앞에 비치된 A2 수거 상자에 모아주세요.

아래 “다음” 버튼을 누르시면 **정답의 총 개수가 공개** 됩니다.

무작위로 결정된 상대보다 맞춘 개수가 많아 **이길 경우는 정답 개수\*2천원**이 확보되며,

**질 경우(0원)**는 아무런 보수도 확보되지 않습니다.

Experiment A2 has just ended. Please submit your envelope and tables to the experimenter.

If you press “Next” button in your computer, you will be informed of the number of correct answers.

If you solve more tables correctly than your partner, you will earn 2000 KRW times the number of correct answers. If you lose, you will earn nothing.

## 실험 A3

# 선택 : 성과제 vs 경쟁제

- ❖ 세 번째 단계도 이전 두 단계와 동일하게 5분 안에 20개의 문제를 풀게 됩니다.
- ❖ 여기서 보수 제도는 1단계 성과제와 2단계 경쟁제 중 선생님께서 선택하신 방법에 따라 결정됩니다.
- ❖ 주목하실 것은 보수제도 선택 전에 선생님께 보너스 점수를 제공합니다.  
보너스는 선생님의 선택에 따라 무작위로 결정되며, 선생님께서 맞추신 개수에 보너스 점수를 합산한 것이 선생님께서 맞춘 최종 개수가 됩니다.
- ❖ 이후 선생님께서 선택하신 성과제, 경쟁제 방법에 따라 이후 3단계 보수가 책정됩니다.

### Experiment A3: Choice between piece-rate scheme and tournament scheme

In the third stage, you will again solve 20 tables in 5 minutes as before. You will be asked to select an incentive scheme between the piece-rate scheme (A1) and the tournament scheme (A2).

Note that you will receive a bonus point before making a choice of an incentive scheme. Your bonus point will be randomly selected. The final number of correct answers in this stage is the number of correct answers you make plus your bonus point.

After observing your bonus point, you will be asked to choose between the piece-rate scheme and the tournament scheme.

## 보너스 점수의 결정

- ❖ 보너스 점수는 선생님의 선택에 따라 무작위로 결정됩니다.
- ❖ 아래 예에서 보시는 것처럼 컴퓨터에는 0~10까지 각각의 번호에 보너스 점수가 부여되어 있습니다.  
(아래의 점수들은 설명을 위한 예시이며 실제와는 다릅니다.)

### [보너스 예시]

| 가)  | 나) | 다) | 라) | 마) | 바) | 사) | 아) | 자) | 차) | 카) |
|-----|----|----|----|----|----|----|----|----|----|----|
| 10점 | 8점 | 7점 | 2점 | 4점 | 0점 | 1점 | 9점 | 3점 | 5점 | 6점 |

- ❖ 예를 들어, 선생님께서 ②번을 선택하시면, 8점의 보너스 점수가 부여됩니다.
- ❖ 아래 문항에 선생님께서 뽑고 싶으신 번호를 뽑아주세요.  
각 번호에 따라 결정되는 보너스 점수는 아무도 모르며,  
선생님 선택이 완료되면 몇 점의 점수가 부여되는지 공개됩니다.

### Selection of a bonus point

Your bonus point will be randomly selected.

As shown below as an example, the computer randomly assigns bonus points from 0 to 10. (Note that it is an illustrative example and is different from the actual selection of your bonus point.)

For instance, if you selected number (2), you will be given the bonus point 8.

Please select a number between 0 and 10 as you wish. No one knows which number is linked to a particular bonus point. Once you select a number, the computer will inform you of your bonus point.

### A3 보수 결정 : ① 성과제 선택 시

- ❖ 성과제를 선택하게 되면, 선생님께서 (맞춘 개수+보너스 점수) \* 1천원을 받게 됩니다.

(보너스 점수+정답의 개수) \* 1천원

보너스 3점, 정답 3개면 총 6개 6,000원

보너스 3점, 정답 12개면 총 15개 15,000원

### A3 보수 결정 : ② 경쟁제 선택 시

- ❖ 무작위로 선택된 상대방과 경쟁해 이기면 점수 \* 2천원을 받고, 지면 보수가 책정되지 않습니다.  
경쟁자는 2단계에서 결정된 사람과 동일하며, 그 상대방이 2단계에서 맞춘 정답의 수로 경쟁합니다.
- ❖ 결국, 상대방은 보너스 점수가 없고 선생님만 보너스 점수가 있습니다.
- ❖ 단, 2단계 결과에는 아무런 영향을 주지 않습니다. 2단계의 승패와 금액은 모두 동일하며,  
2단계 상대방의 점수는 현재 단계 선생님 점수와 비교 대상으로만 사용이 됩니다.

내 점수  
이번에 맞춘 개수 + 보너스 점수

VS

상대 점수  
2단계에서 짝지어진 상대방의 2단계 점수

#### Experiment A3: Earnings when you selected the piece-rate scheme

If you chose the piece-rate scheme, your earnings will be given by the number of correct answers times 1000 KRW.

#### Experiment A3: Earnings when you selected the tournament scheme

If you won against your randomly assigned partner, you will receive 2000 KRW for each correct answer. If you lost, you will earn nothing.

Your partner is the same person matched to you in Experiment A2. Your partner will compete with you with the number of correct answers that your partner solved in Experiment A2. That is, your partner will have no bonus point, whereas you have a bonus point.

Note that this stage will not affect the earnings of Experiment A2 for you and your partner. The number of correct answers that your partner solved in Experiment A2 is only used to determine who wins if you selected the tournament scheme.

- ❖ 잠시 후 문제 봉투를 나누어 드리겠습니다.
- ❖ 진행자가 '시작'을 외치면 총 5분 동안 문제를 푸시고 정답을 입력해주세요.  
시작을 외치기 전 봉투를 미리 개봉하면 실격 처리 됩니다.
- ❖ 5분이 모두 지나면 봉투는 한꺼번에 모두 회수하겠습니다.

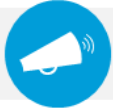

진행요원들은 숫자표 봉투 A3을 나눠주세요.

- ❖ 먼저, 봉투에 본인 이름과 ID를 정확히 적어주세요.
- ❖ 그럼, 이제 시작을 외치면 '다음'을 누르시고 봉투를 개봉해 5분간 문제풀이를 시작하게 됩니다.

## “시작”

You will soon be given an envelope containing 20 tables for this stage. If the experimenter announces "Start", you can start counting zeros and submitting your answers in 5 minutes.

You will be disqualified if you open your envelope before the experimenter announces "Start." Answers you submit within 5 minutes in the computer will be only counted.

The experimenter will show you a timer through a beam projector and will announce "one minute remaining" when 4 minutes pass.

[The experimental assistants distribute envelopes to subjects]

Please write down your name and ID on the envelope. The experimenter is about to announce "Start."

실험A3을 종료합니다.

진행자에게 문제지와 봉투를 제출해주세요.

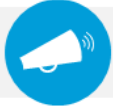

진행요원들은 담당구역의 봉투를 신속하게 걷어주세요.  
앞에 비치된 A3 수거 상자에 모아주세요.

아래 “다음” 버튼을 누르시면 **정답의 총 개수**가 **공개** 됩니다.

Experiment A3 has just ended. Please submit your envelope and tables to the experimenter.

If you press “Next” button in your computer, you will be informed of the number of correct answers.

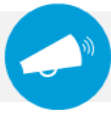

진행요원들은 칸막이를 제거해주세요.

**보수책정 1단계 실험을  
모두 완료하셨습니다.**

**3개의 결과 중 최종 보수는  
다음 추가 실험 진행 후 선생님의 제비뽑기를  
통해 확정됩니다.**

보수책정  
**1**

실험 A1  
실험 A2  
실험 A3

성과제 결과  
경쟁제 결과  
성과제 or 경쟁제 결과

제비  
뽑기

1단계  
최종보수

The experiment has ended.

You will make a lottery to select one of the three stages—A1, A2, and A3. It will be counted for your final earnings.

## 추가 Track ① 기대측정 실험

- ❖ 이번에는 선생님께서 경쟁을 했을 때 본인이 이겼을 가능성을 예측하시고,  
그 결과가 얼마나 정확한지에 따라 추가 보수를 지급하는 실험입니다.
- ❖ 이 결과에 따라 **2천원의 추가 보수**가 확정될 수 있습니다.

### Extra track (1): Elicitation of winning probability

You will now be asked to guess your winning probability when you compete with your partner. You will earn 2000 KRW depending on how accurate your guess is.

## 경쟁에서 이길 확률

- ❖ 앞서 개인실험 3단계(선택: 성과제 vs 경쟁제)에서 선생님의 정답 수와 보너스 숫자는 아래와 같습니다.
- ❖ 해당 단계에서 보너스를 합친 선생님의 숫자가 경쟁 상대가 되는 2단계 상대방(보너스가 없이 맞춘 개수만 있는)을 이길 확률이 얼마나 될지 아래 문항에서 선택해 주세요.

내 점수  
개인 3단계에 맞춘 개수 + 보너스 점수

VS

상대 점수  
2단계에서 짝지어진 상대방의 2단계 점수

- ❖ 이 중에는 해당 단계에서 경쟁제를 선택하신 분들도 있고, 경쟁 없이 성과제를 선택하신 분들도 있습니다. 후자의 경우는 '만약 경쟁을 했으면, 이길 확률이 얼마나 됐을까' 가정으로 응답해 주시면 됩니다.
- ❖ 이 단계는 선생님의 예측이 실제 결과와 얼마나 가까운가가 중요한 기준입니다. 따라서, 최선의 방식은 이길 수 있었을까라는 기대치를 정확히 입력하는 것이 가장 중요합니다.

### Probability of winning in the tournament

In the previous experiment A3, the number of correct answers and your bonus point are as below.

Please guess your winning probability in that experiment. Please note that you competed against your partner with the number of correct answers you solved in that experiment plus your bonus point, while the number of correct answers your partner solved in the experiment A2 was used.

You may have chosen the piece-rate scheme. In that case, please guess your winning probability if you have chosen the tournament.

It is important how close your guess is to the real outcome. Therefore, you are asked to guess as accurately as possible your winning probability.

## 기대의 예측 오류 계산

- ❖ 방금 선생님께서 이겼을 것이라고 예측하신 것이 틀릴 가능성을 **예측 오류**라고 합니다.
- ❖ 예측 오류는 아래와 같이 이긴 경우는  $(1 - \text{예측치})$ 의 제곱으로, 진 경우는  $(\text{예측치})$  제곱으로 계산됩니다.

|    | 이길 확률 |   | 실제로 이긴 경우        | 실제는 진 경우     |
|----|-------|---|------------------|--------------|
| 수식 | $x\%$ | → | $(1-x)^2$        | $x^2$        |
| 예시 | 20%   | → | $(1-0.2)^2=0.64$ | $0.2^2=0.04$ |

- ❖ 선생님의 예측오류는 상대방이 결정되어야 할 수 있으므로, 실험 종료 후 상황판에 공개됩니다.
- ❖ 이후 컴퓨터의 무작위 프로그램을 통해 0부터 1까지 숫자가 하나 결정되며,  
이것보다 선생님의 **예측오류가 작으면 2천원**을 추가로 받고, **높으면 0원**을 받게 됩니다.

### Computing prediction error

The prediction error is referred to as a chance of your guess being wrong. Given  $x\%$  as your winning probability guess, the prediction error is computed as  $(1 - x)^2$  if you actually won and as  $(x)^2$  if you lost.

Your prediction error will be announced after your partner is determined.

The computer will randomly select a real number between 0 and 1. If your prediction error is smaller than a randomly selected number, you will receive 2000 KRW. Otherwise, you will receive nothing.

## PART C

# 보수책정 3단계

- ❖ 지금부터는 이제까지 선택한 것과 전혀 다른 실험이 진행되며, 개인 과제입니다.
- ❖ 이 단계에서는 확률에 따라 금액이 다른 두 개의 복권 중 한 개의 복권을 선택하는 의사결정 실험입니다.
- ❖ 이 단계에서 선생님이 받아가실 금액은 선생님의 의사결정에 따라 달라지며,  
역시 실험과 설문이 모두 끝나고 나가실 때 기본 답례금과 앞서 받으신 보수에 더해 받아가시게 됩니다.
- ❖ 그럼, 실험 요령을 순서대로 설명 드리겠습니다.

### Part C: Lottery choice experiment

You will participate to a different experiment in which you are asked to choose between two lotteries. You will receive additional earnings from this part of the experiment. We will explain the detail of the experiment.

## 첫 단계 : 복권의 선택

- ❖ 선생님께서 두 개의 복권 중 하나의 복권을 선택하게 됩니다.
- ❖ 복권1을 택하면 5천원 혹은 4천원을 받을 수 있으며, 해당 금액이 선택될 확률은 10% : 90%입니다.  
반대로, 복권2를 택하면 1만원을 받거나 하나도 못 받으며, 해당 금액이 선택될 확률은 1:9로 동일합니다.

|    |       | 복권1   |       |    |  | 복권2    |     |
|----|-------|-------|-------|----|--|--------|-----|
| C1 | 받을 금액 | 5,000 | 4,000 | VS |  | 10,000 | 0   |
|    | 받을 확률 | 10%   | 90%   |    |  | 10%    | 90% |

복권1 선택시

5천원 받을 확률이 10%, 4천원 받을 확률이 90%

복권2 선택시

1만원 받을 확률이 10%, 하나도 못받을 확률이 90%

- ❖ 이러한 복권의 선택을 총 10번하게 되는데, 각 복권의 금액은 동일하며 확률만 달라집니다.  
아래의 경우는 확률이 100%이기 때문에 반드시 복권 1을 택하면 5천원, 2를 택하면 1만원을 받습니다.

|     |       | 복권1   |       |    |  | 복권2    |    |
|-----|-------|-------|-------|----|--|--------|----|
| C10 | 받을 금액 | 5,000 | 4,000 | VS |  | 10,000 | 0  |
|     | 받을 확률 | 100%  | 0%    |    |  | 100%   | 0% |

### Lottery choice experiment

You will be asked to choose between two lotteries in each of 10 lottery choice problems. For instance, if you select Lottery 1, you will earn 5000 KRW with 10% probability or 4000 KRW with 90% probability. If you select Lottery 2, you will earn 10000 KRW with 10% probability or nothing with 90% probability.

You will make choices in such 10 problems where money amounts are fixed and probabilities change. For instance, in the following problem where one of the outcomes is given with 100% probability, you will earn for sure 5000 KRW if you select Lottery 1 and 10000 KRW if you select Lottery 2.

## 첫 단계 : 복권의 선택

❖ 아래가 실제 문제지입니다.

복권1을 선택하면 받을 수 있는 금액은 5천원, 4천원 두 가지로 모두 동일하고,

복권2를 선택하면 받을 수 있는 금액은 1만원, 0원 두 가지로 모두 동일합니다.

❖ 다만 다음 문항일수록 5천원 혹은 1만원을 받을 수 있는 확률이 높아지고, 반대는 낮아집니다.

|            | 복권1   |       | 복권2    |     |
|------------|-------|-------|--------|-----|
| 받을 금액      | 5,000 | 4,000 | 10,000 | 0   |
| C1. 받을 확률  | 10%   | 90%   | 10%    | 90% |
| C2. 받을 확률  | 20%   | 80%   | 20%    | 80% |
| C3. 받을 확률  | 30%   | 70%   | 30%    | 70% |
| C4. 받을 확률  | 40%   | 60%   | 40%    | 60% |
| C5. 받을 확률  | 50%   | 50%   | 50%    | 50% |
| C6. 받을 확률  | 60%   | 40%   | 60%    | 40% |
| C7. 받을 확률  | 70%   | 30%   | 70%    | 30% |
| C8. 받을 확률  | 80%   | 20%   | 80%    | 20% |
| C9. 받을 확률  | 90%   | 10%   | 90%    | 10% |
| C10. 받을 확률 | 100%  | 0%    | 100%   | 0%  |

### Lottery choice problem

The following is the list of binary lottery choices that you will face. Note that Lottery 1 always uses (5000 KRW, 4000 KRW) and Lottery 2 always uses (10000 KRW, 0 KRW).

Please note that a lottery choice problem further down in the list involves a higher probability of winning 5000 KRW or 10000 KRW.

## 두번째 단계 : 받을 확률의 추천

❖ 다음 단계는 선생님께서 선택한 10개의 복권 중 한 개의 복권을 추천하는 단계입니다.

앞서와 마찬가지로 번호를 고르면, 컴퓨터에 입력된 번호에 따라 선생님이 받을 복권이 결정됩니다.

### [C1~C10 복권 결정 예시]

| ①           | ②           | ③            | ④           | ⑤           | ⑥           | ⑦           | ⑧           | ⑨           | ⑩           |
|-------------|-------------|--------------|-------------|-------------|-------------|-------------|-------------|-------------|-------------|
| C3의<br>선택복권 | C7의<br>선택복권 | C10의<br>선택복권 | C8의<br>선택복권 | C4의<br>선택복권 | C5의<br>선택복권 | C1의<br>선택복권 | C2의<br>선택복권 | C9의<br>선택복권 | C6의<br>선택복권 |

❖ 예를 들어, 선생님께서 ②번을 선택하시면, C7 단계에서 선택하신 선생님의 복권이 확정됩니다.

❖ 아래처럼 복권2를 이전 단계에서 고르셨다면, 만원 받을 확률이 70%, 받지 못할 확률이 30%입니다.

|           | 복권1   |       | 복권2    |     |
|-----------|-------|-------|--------|-----|
| 받을 금액     | 5,000 | 4,000 | 10,000 | 0   |
| C7. 받을 확률 | 70%   | 30%   | 70%    | 30% |

### Selection of a lottery choice problem that counts

Once you completed your choices in the 10 lottery choice problems of the list, you will be asked to participate in the random selection of one of the problems that will count for your earnings.

For instance, if the seventh problem is randomly selected, your choice in the seventh problem will count for the determination of your earnings in this experiment.

### 세번째 단계 : 최종 복권 추첨

- ❖ 이제 최종적으로 복권을 추첨합니다.
- ❖ 다시 한 번 무작위로 번호를 뽑게 되며, 1~10까지 숫자가 아래처럼 무작위로 입력되어 있습니다.

[복권 추첨 예시]

| ① | ② | ③  | ④ | ⑤ | ⑥ | ⑦ | ⑧ | ⑨ | ⑩ |
|---|---|----|---|---|---|---|---|---|---|
| 6 | 5 | 10 | 2 | 4 | 8 | 7 | 3 | 9 | 1 |

- ❖ 각 번호는 당첨의 확률을 의미하며, C1 단계 복권1(5천원 10%, 4천원 90%)을 선택하셨다면, 1이 당첨되면, 5천원, 2~10이 당첨되면 4천원을 받게 됩니다.
- ❖ 앞선 예에 이어, C7 단계의 복권 2를 앞 단계에서 선택했고,
- ❖ 이 단계에서 선생님께서 ②번을 선택해 5번(50%)이 결정됐다면, 70%이내로 당첨되어 1만원을 받습니다.

#### Determination of your earnings

Given the random selection of a decision problem that counts for your earnings, your earnings will be randomly determined by your lottery choice of that problem. For instance, if the lottery of 5000 KRW with 10% probability and 4000 KRW with 90% probability is considered for your final earnings, you will participate in a random draw to determine your actual earnings.

## 추가 Track ② 인지력 퀴즈

- ❖ 지금부터 총 10분 동안 도형과 관련된 24개 문제를 푸시게 됩니다.
- ❖ 앞서 진행하신 실험과 다르게, 지금부터 문제를 푸신 결과는 선생님의 답례금 책정에 영향을 주지 않습니다.

Extra Track (2): cognitive test quiz

You are about to solve 24 figural reasoning quizzes in 10 minutes. Differently from the experiment to which you participated just before, you will not receive any earnings from this part.

## 인지력 퀴즈 예시

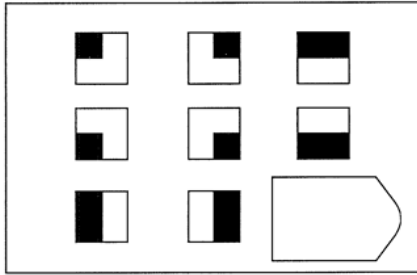

- ❖ 선생님께서 받게 되실 조사표에서 왼쪽 상단과 같은 9개의 도형으로 이루어진 그림을 보시게 됩니다.
- ❖ 각 도형은 왼쪽에서 오른쪽, 그리고 위에서 아래로 일정한 규칙을 가지고 있고, 이 규칙을 이해하셔서 오른쪽 하단 빈 칸에 들어갈 도형을 맞춰야 합니다.

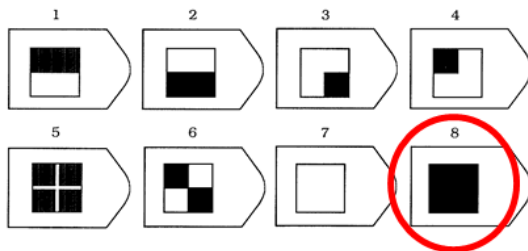

- ❖ 보기는 8개가 제시되며, 그 중 정답을 골라주시면 됩니다.
- ❖ 왼쪽 예시 문항의 정답은 8번입니다.

Example of cognitive test

You will see a picture of 9 diagrams as shown in the upper left corner.

Each diagram follows a certain rule, from left to right and from top to bottom. You will be asked to figure out this rule and match a shape that fits into the lower right empty space.

You will be presented with 8 possible choices. Please select the correct answer.

The answer to this example is 8.
